# Supplementary material for: Street TryOn: Learning In-the-Wild Virtual Try-On from Unpaired Person Images
Source: arXiv:2311.16094 source file (2024-07-16)
Supplement: Supplementary file 1 [file more_experiments.tex]

\begin{table*}[!htb]
\centering
\caption{
\textbf{Comparsions with prior work in same-domain and cross-domain tests.} 
PASTAGAN++ (released) is the officially released model trained on UPT dataset~\cite{xie2021pastagan}, which contains unpaired model images. We train PASTAGAN++ (street) on the training split of the Street TryOn dataset with the default settings.
}

\resizebox{\textwidth}{!}{

\begin{tabular}{|c||ccc||c|c|c|}
\hline
\multirow{5}*{}
     & \multicolumn{3}{c||}{Training Settings}

     & Model2Model
     & Model2Street
     & Street2Street \\ 
     & \small{paired}
     & \small{garment src}
     & \small{person src}
     & \small{FID $\downarrow$} 
     & \small{FID $\downarrow$}
     & \small{FID $\downarrow$}
     \\\hline

PastaGAN++~\cite{xie2022pastagan++} (released)
& $\times$ & model & model  
& 13.848
& 71.090
& 67.016
\\ 

PastaGAN++ ~\cite{xie2022pastagan++}  (street)
& $\times$ & street & street  
& 40.841
& 70.461
& 67.088
\\ \hline

%ours (w/o SD)
%& paired & shop & model 
%%&  &  & 
%%& 64.046 & 71.512 & 72.408
%%\\ 

ours (1)
& \checkmark & shop & model 
& 10.961
& \textbf{34.050} & 33.165
\\ 

ours (2)
& $\times$ & model & model 
& 11.040 & 34.434 & 33.742 \\ 

ours (3)
& $\times$ & street & street  
& \textbf{10.214} & 34.191 & \textbf{33.039}
 \\
\hline

\end{tabular}
}

\label{tab:pastagan_table}
\end{table*}
\section{Additional Experiments for PASTAGAN++}

PASTAGAN++~\cite{xie2022pastagan++} is the state-of-the-art method among the prior work that learns virtual try-on from unpaired images. The main paper shows that the PASTAGAN++ trained with model images is not robust enough to generalize to street2street try-on task and cross-domain try-on tasks.

Here, we run an additional experiment that trains PASTAGAN++ from scratch with the street images in the proposed Street TryOn benchmark. The results in Tab~\ref{tab:pastagan_table} and Fig.~\ref{fig:person2person_comparison} show that PASTAGAN++ cannot deal with street images (i.e., casual images of people against cluttered backgrounds). As a StyleGAN2-based method, PASTAGAN++ learns a latent space to encode the data distribution for image patches. Although such a distribution can be learned for relatively structural data like person images with a clean background, it is hardly possible to learn a highly diverse distribution~\cite{sauer2022styleganXL} to represent the complex background for in-the-wild images. Therefore, the PASTAGAN++ trained with street images is struggling with the background reconstructions and cannot generate the street try-on images as faithfully as our method does.

\begin{figure*}
    \centering
    \includegraphics[width=\textwidth]{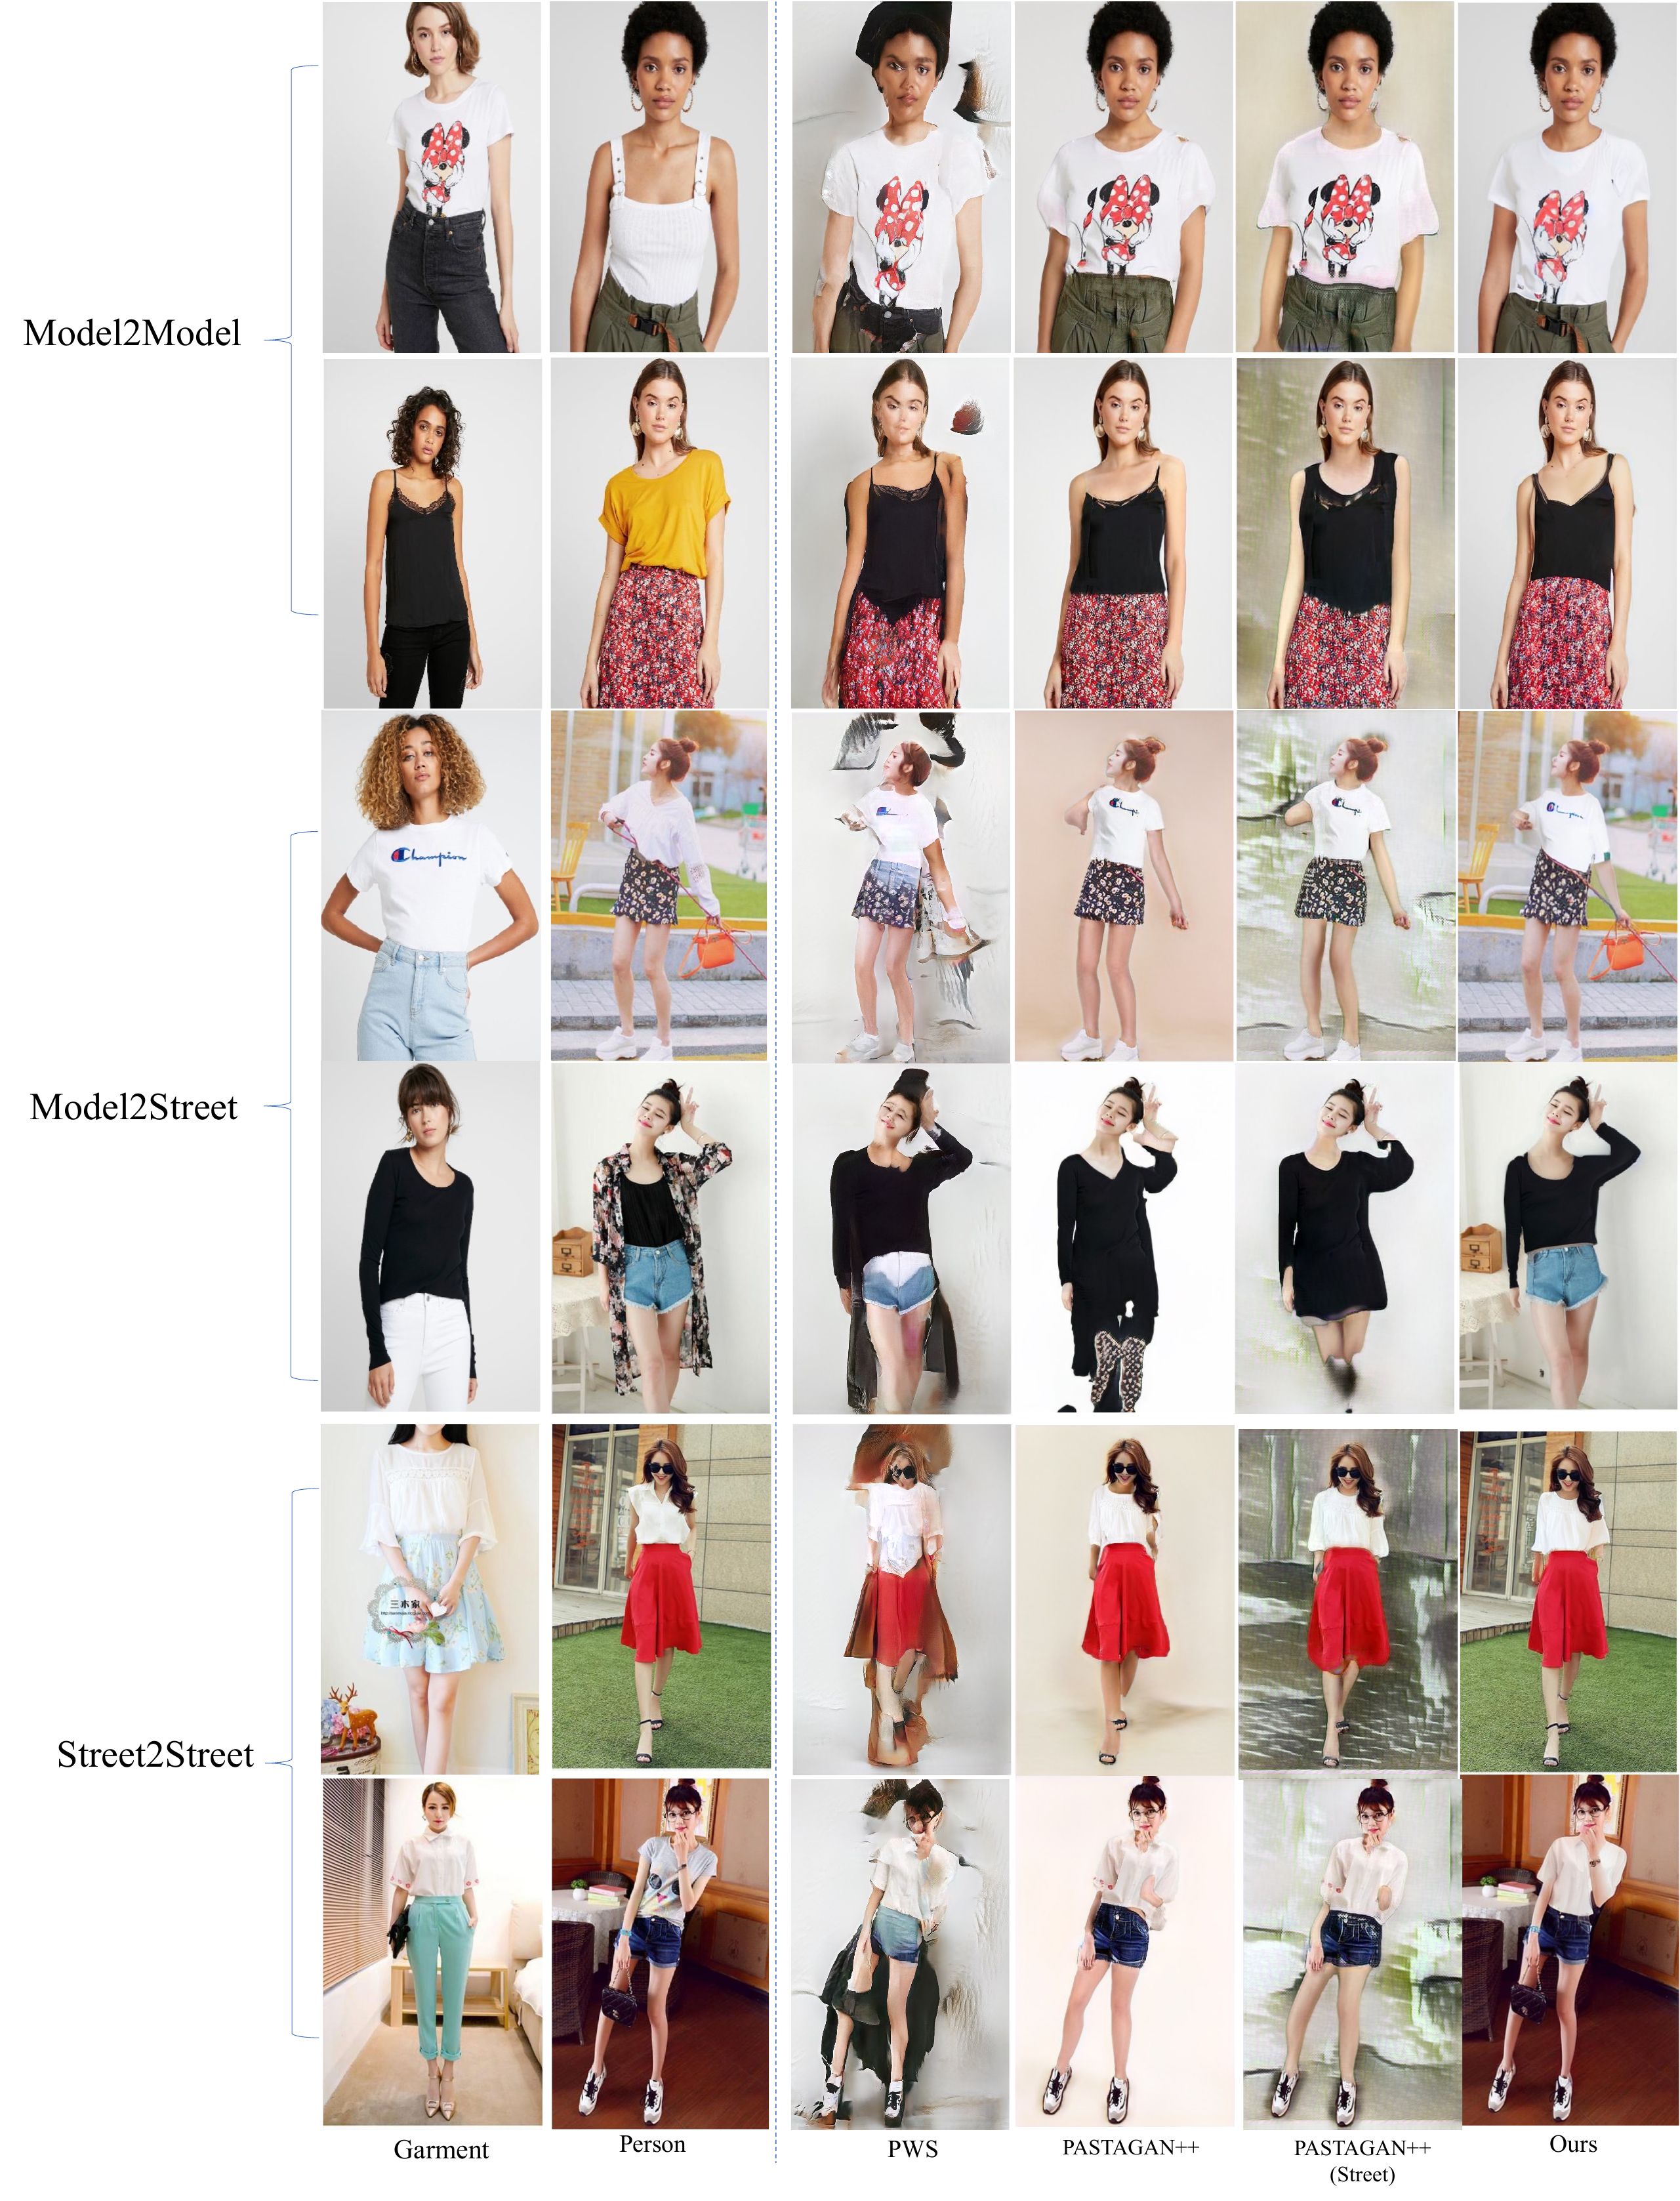}
    \vspace{-3mm}
    \caption{Visual Comparisons with PWS~\cite{albahar2021posewithstyle} and PASTAGAN++~\cite{xie2022pastagan++}. }
    \label{fig:person2person_comparison}
\end{figure*}

\section{Additional Ablation Study}
We report an ablation study that separately analyzes the effects of our DensePose warping and inpainting-based compositing. 
We take FS-VTON~\cite{he2022styleflow}, a non-diffusion-based method with separate warping and refinement modules, whose warping module is trained using paired studio images. We individually replace our warping and refinement modules with theirs. Here, our method is trained with paired data on VITON-HD for a fair comparison. As shown in  Fig.\ref{fig:ablation_robustness}, both our proposed warping module and the diffusion

\begin{figure}
\vspace{-5mm}
\centering

\begin{minipage}{0.7\textwidth}
\centering
      \includegraphics[width=\textwidth]{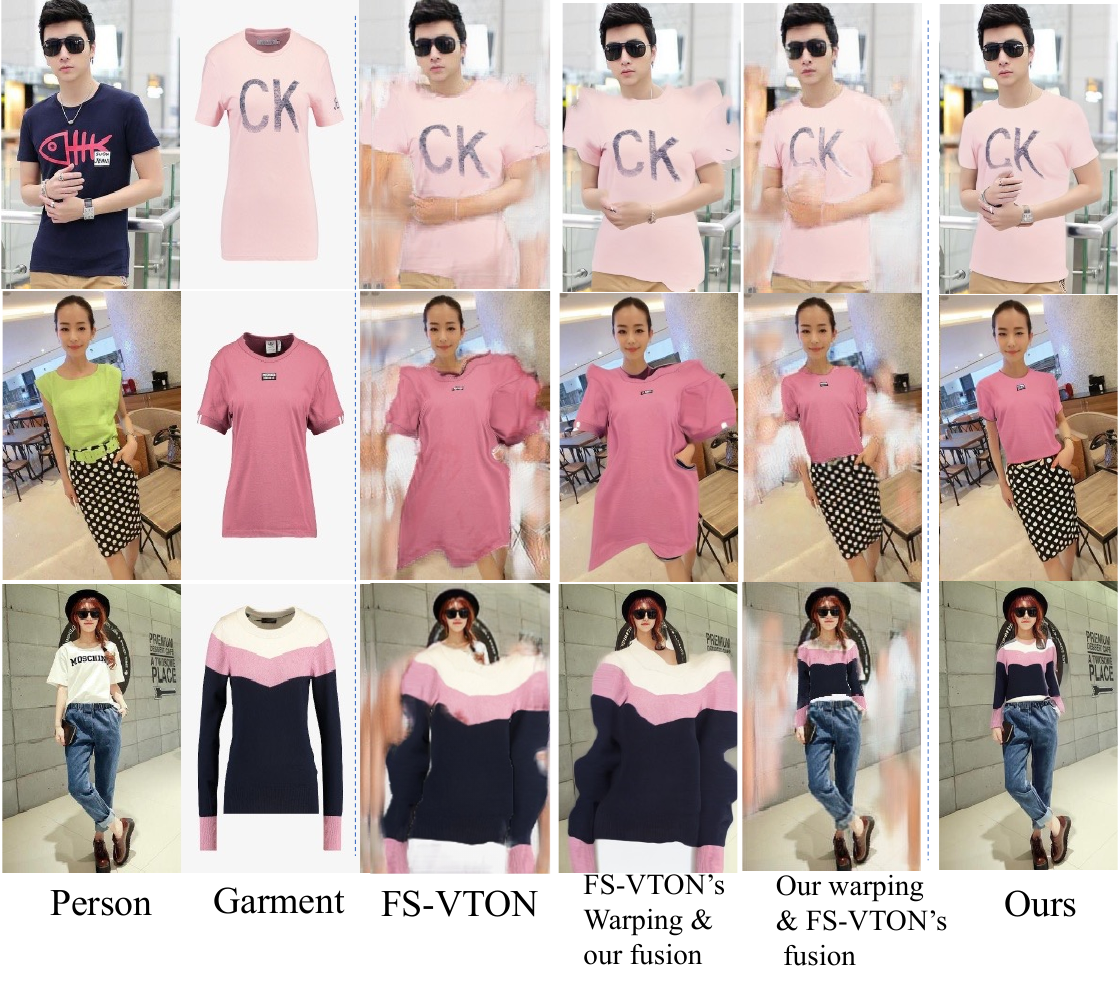} 
      %\subcaption{Visual Results.}

\end{minipage}
%\vspace{-5mm}
\begin{minipage}[c]{\textwidth}
%\vspace{-240px}
%\hspace{90px}
\centering
\resizebox{0.7\textwidth}{!}{

    \begin{tabular}[t]{|cc||c|}
        \hline
        Warping Method & Fusion Method  & Shop2Street (FID)  \\ \hline
        FS-VTON & FS-VTON & 90.972 \\
        FS-VTON & SD-inpainting & 77.456 \\
        ours & FS-VTON &   64.046 \\
        ours & SD-inpainting &  \textbf{33.819} \\
        \hline
    \end{tabular}
    }
    \vspace{-3mm}
\end{minipage}

\caption{
Comparison with warping and compositing (fusion) modules of FS-VITON~\cite{he2022styleflow} in FID. 
%We use the officially released model weights for both components of FS-VTON in all the experiments at 256x192. 
\textbf{Top:} Visual Results.
\textbf{Bottom:} Quantitative Results. 
 \label{fig:ablation_robustness}
 }

\end{figure}
 %\vspace{-5mm}
