# Supplementary material for: Street TryOn: Learning In-the-Wild Virtual Try-On from Unpaired Person Images
Source: arXiv:2311.16094 source file (2024-07-16)
Supplement: Supplementary file 3 [file main.tex]

%\tableofcontents
\input{supp/dataset_filtering_details}
\newpage
\input{supp/cosine_noise_details}

\input{supp/diffusion_inpainting_details}
\input{supp/more_results}
