# Supplementary material for: Street TryOn: Learning In-the-Wild Virtual Try-On from Unpaired Person Images
Source: arXiv:2311.16094 source file (2024-07-16)
Supplement: Supplementary file 4 [file pastgan_table.tex]

\begin{table*}[!htb]
\centering
\caption{
\textbf{Comparsions with prior work in same-domain and cross-domain tests.} 
PASTAGAN++ (released) is the officially released model trained on UPT dataset~\cite{xie2021pastagan}, which contains unpaired model images. We train PASTAGAN++ (street) on the training split of the Street TryOn dataset with the default settings.
}

\resizebox{\textwidth}{!}{

\begin{tabular}{|c||ccc||c|c|c|}
\hline
\multirow{5}*{}
     & \multicolumn{3}{c||}{Training Settings}

     & Model2Model
     & Model2Street
     & Street2Street \\ 
     & \small{paired}
     & \small{garment src}
     & \small{person src}
     & \small{FID $\downarrow$} 
     & \small{FID $\downarrow$}
     & \small{FID $\downarrow$}
     \\\hline

PastaGAN++~\cite{xie2022pastagan++} (released)
& $\times$ & model & model  
& 13.848
& 71.090
& 67.016
\\ 

PastaGAN++ ~\cite{xie2022pastagan++}  (street)
& $\times$ & street & street  
& 40.841
& 70.461
& 67.088
\\ \hline

%ours (w/o SD)
%& paired & shop & model 
%%&  &  & 
%%& 64.046 & 71.512 & 72.408
%%\\ 

ours (1)
& \checkmark & shop & model 
& 10.961
& \textbf{34.050} & 33.165
\\ 

ours (2)
& $\times$ & model & model 
& 11.040 & 34.434 & 33.742 \\ 

ours (3)
& $\times$ & street & street  
& \textbf{10.214} & 34.191 & \textbf{33.039}
 \\
\hline

\end{tabular}
}

\label{tab:pastagan_table}
\end{table*}
